# Supplementary material for: Nonlinear dynamics and emergent statistical regularity in classical Lennard-Jones three-body system upon disturbance
Source: arXiv:2312.05186 source file (2023-12-08)

# Supplemental Materials

Zhenwei Yao\*

*School of Physics and Astronomy, and Institute of Natural Sciences,*

*Shanghai Jiao Tong University, Shanghai 200240, China*

In this document, we present technical details of the numerical approach, and supplemental information about trajectory evolution, frequency spectrum analysis of kinetic energy and statistical analysis of particle trajectories.

## I. TECHNICAL DETAILS

In this section, we present technical details in the numerical integration of the equations of motion, including the formulation of the initial conditions, the derivation of the dynamical matrix  $K$ , and more information about the conservation laws.

### A. Initial conditions

The initial conditions for the three-body system are formulated either by imposing initial displacements or by specifying initial velocities. In the former case, the particles are disturbed by a random displacement  $\vec{r}_i$  with fixed magnitude  $b \times a$  ( $a$  is the balance distance of the L-J potential) and random orientations  $\theta_i$  with respect to the  $x$  axis, where  $i = 1, 2, 3$ .  $\theta_i$  are independent uniform random variables in  $[0, 2\pi)$ .

For convenience in the investigation of the statistical property of the three-body system, we work in the frame of reference where both the total momentum and angular momentum are zero. To this end, the initial condition is specified in terms of initial velocities. Specifically, the origin of the coordinates is set at the center of the equilibrium triangular configuration of the particles, where the three particles are located at  $(-a/2, -\sqrt{3}a/6)$ ,  $(a/2, -\sqrt{3}a/6)$ , and  $(0, \sqrt{3}a/3)$ , respectively. The initial velocities are subject to the follow-

---

\*Electronic address: zyao@sjtu.edu.cn

ing constraints:

$$\begin{aligned}\sum_{i=1}^3 \vec{v}_i &= 0, \\ \sum_{i=1}^3 \vec{r}_i \times \vec{v}_i &= 0.\end{aligned}\tag{1}$$

The motion is confined in the x-y plane, so Eqs.(1) constitute three constraints for the six components of the initial velocities. Given the components of the initial velocities  $\{v_{1x}, v_{1y}, v_{2y}\}$ , the other three components can be determined.  $v_{1x}$ ,  $v_{1y}$  and  $v_{2y}$  are expressed in terms of the fixed amplitude  $v_{\text{ini}}$  and random orientation. Specifically,  $v_{1x} = v_{\text{ini}} \cos \theta_1$ ,  $v_{1y} = v_{\text{ini}} \sin \theta_1$ , and  $v_{2y} = v_{\text{ini}} \sin \theta_2$ .  $\theta_i$  are uniform random variables in  $[0, 2\pi)$ . The characteristic initial speed  $v_{\text{ini}}$  specifies the strength of the initial disturbance.

## B. The dynamical matrix $K$

In the linear regime, the  $\vec{f}(\vec{X})$  term in the equations of motion in the main text becomes:

$$f_\alpha(\vec{X}) = -\beta_0 K_{\alpha\beta} X_\beta,\tag{2}$$

$\alpha, \beta = x, y$ .  $\vec{X} = \{r_{i\alpha}\}$ , where  $r_{i\alpha}$  is the  $\alpha$ -component of the displacement of particle  $i$ . The complete expression for the dynamical matrix  $K$  is analytically derived and presented below:

$$K = \begin{pmatrix} \frac{5}{4} & \frac{\sqrt{3}}{4} & -1 & 0 & -\frac{1}{4} & -\frac{\sqrt{3}}{4} \\ \frac{\sqrt{3}}{4} & \frac{3}{4} & 0 & 0 & -\frac{\sqrt{3}}{4} & -\frac{3}{4} \\ -1 & 0 & \frac{5}{4} & -\frac{\sqrt{3}}{4} & -\frac{1}{4} & \frac{\sqrt{3}}{4} \\ 0 & 0 & -\frac{\sqrt{3}}{4} & \frac{3}{4} & \frac{\sqrt{3}}{4} & -\frac{3}{4} \\ -\frac{1}{4} & -\frac{\sqrt{3}}{4} & -\frac{1}{4} & \frac{\sqrt{3}}{4} & \frac{1}{2} & 0 \\ -\frac{\sqrt{3}}{4} & -\frac{3}{4} & \frac{\sqrt{3}}{4} & -\frac{3}{4} & 0 & \frac{3}{2} \end{pmatrix}.\tag{3}$$

The six eigenvalues of the  $K$  matrix are:  $\{3/2, 3/2, 3, 0, 0, 0\}$ . The frequency of the normal mode corresponding to the eigenvalue  $\lambda$  is:  $\omega_\lambda = \sqrt{\beta_0 \lambda / m}$ .  $\omega_{\lambda_1} = 2^{5/6} 3^{3/2} \approx 9.3$ , and  $\omega_{\lambda_2} = 2^{4/3} 3^{3/2} \approx 13.1$ .

| $t$   | $E_t$    | $L_z (\times 10^{-11})$ | $P_x (\times 10^{-10})$ | $P_y (\times 10^{-10})$ | $R_x (\times 10^{-6})$ | $R_y (\times 10^{-6})$ |
|-------|----------|-------------------------|-------------------------|-------------------------|------------------------|------------------------|
| 250   | -2.94931 | 6.23                    | 1.41                    | 0.29                    | 0.005                  | 0.002                  |
| 2500  | -2.94936 | 8.55                    | 3.06                    | -2.22                   | 0.19                   | -0.12                  |
| 5000  | -2.94937 | 10.7                    | 6.52                    | -4.57                   | 0.64                   | -0.38                  |
| 7500  | -2.94936 | 20.6                    | 10.83                   | -6.19                   | 1.34                   | -0.87                  |
| 10000 | -2.94933 | 21.1                    | 8.76                    | -5.72                   | 2.21                   | -1.39                  |
| 12500 | -2.94936 | 27.7                    | 7.95                    | -4.73                   | 2.97                   | -1.82                  |
| 15000 | -2.94931 | 33.0                    | 9.35                    | -2.96                   | 3.76                   | -2.19                  |
| 17500 | -2.94931 | 17.0                    | 6.16                    | -0.96                   | 4.43                   | -2.33                  |
| 20000 | -2.94930 | 12.7                    | 6.71                    | -0.89                   | 4.91                   | -2.44                  |
| 22500 | -2.94938 | 12.7                    | 6.19                    | 0.09                    | 5.44                   | -2.50                  |
| 24500 | -2.94932 | 25.2                    | 9.61                    | 0.20                    | 5.96                   | -2.50                  |

(a)

| $t$   | $E_t$ | $L_z (\times 10^{-6})$ | $P_x (\times 10^{-8})$ | $P_y (\times 10^{-8})$ | $R_x (\times 10^{-6})$ | $R_y (\times 10^{-6})$ |
|-------|-------|------------------------|------------------------|------------------------|------------------------|------------------------|
| 250   | 0.115 | 5.99                   | 1.18                   | -1.29                  | 0.83                   | -0.87                  |
| 2500  | 0.116 | 2.99                   | 1.29                   | -1.75                  | 1.06                   | -9.07                  |
| 5000  | 0.116 | 0.86                   | 1.46                   | -1.68                  | 2.26                   | -2.34                  |
| 7500  | 0.116 | 3.36                   | -1.14                  | -1.68                  | 1.52                   | -3.74                  |
| 10000 | 0.116 | -2.48                  | -1.14                  | 1.82                   | 5.71                   | -2.72                  |
| 12500 | 0.116 | -1.11                  | 2.00                   | 1.82                   | 1.75                   | -1.21                  |
| 15000 | 0.116 | -1.11                  | 2.00                   | 1.82                   | 3.42                   | 3.09                   |
| 17500 | 0.116 | -5.97                  | 2.00                   | -0.36                  | 5.08                   | 6.20                   |
| 20000 | 0.116 | -6.08                  | 2.00                   | -0.36                  | 6.75                   | 3.17                   |
| 22500 | 0.115 | -4.13                  | 8.54                   | -0.36                  | 1.19                   | 1.39                   |
| 24500 | 0.116 | -4.15                  | 8.54                   | -0.36                  | 1.75                   | -2.28                  |

(b)

TABLE I: Variation of some key physical quantities in the long time evolution of the three-body system at varying initial speed.  $v_{\text{ini}} = 0.22$  (a) and 1.12 (b).  $E_t$ ,  $L_z$ ,  $\vec{P}$ , and  $\vec{R}$  are the total energy, angular momentum, momentum, and the position vector of the center of mass.  $h = 5 \times 10^{-4}$ .

### C. Conservation of total energy, momentum and angular momentum

We numerically integrate Eqs.(2) in the main text at fine time step up to a hundred million time steps to ensure the conservation of total energy, momentum and angular momentum in the entire simulation time. In Table I, we list the temporal variation of the following quantities: total energy  $E_t$ , total angular momentum  $L_z$ , total momentum ( $P_x$  and  $P_y$ ) and the location of the center of mass ( $R_x$  and  $R_y$ ). Table I(a) and I(b) are for the cases of varying initial speed:  $v_{\text{ini}} = 0.22$  (a) and 1.12 (b). In both cases, the initial disturbance is sufficiently strong and the system exhibits frequency-mixing phenomenon. The initial values for all the listed quantities are zero except  $E_t$ . Notably, the variation of the total energy is neglectable in comparison with the kinetic energy. The high quality particle trajectories (in

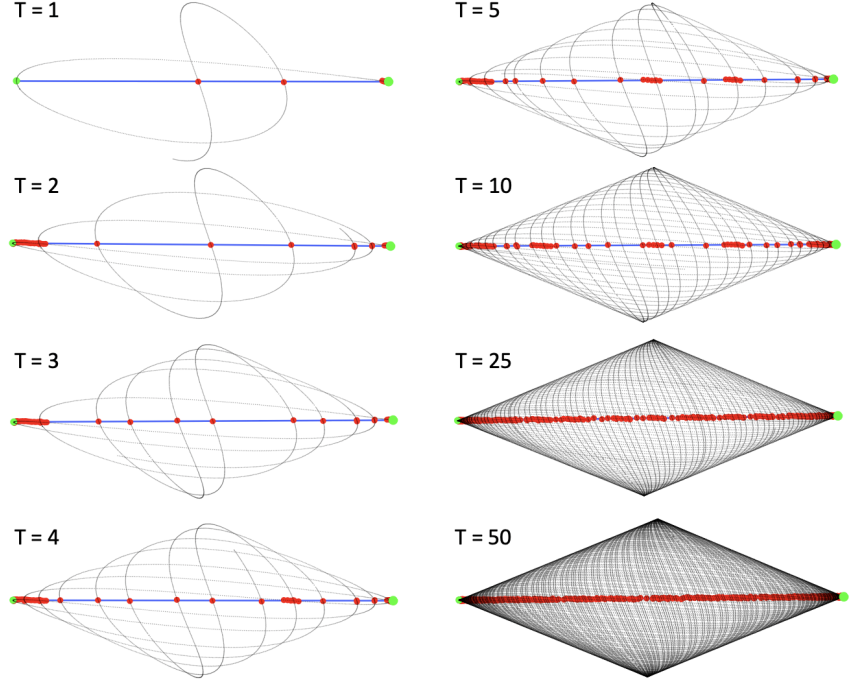

FIG. 1: The trajectories of a particle in the triplet system at varying time interval  $T$ . This figure supplements the trajectory information in Fig.2(a) in the main text. The crossing points of the trajectory and the reference line (blue line) are indicated by red dots; the connecting line of the two furthest points in the trajectory is chosen as the reference line. A point on the trajectory is regarded as a crossing point if its distance to the reference line is less than one thousandth of the length of the reference line.  $b = 0.001$ .

the sense of obeying the conservation laws) constitute the foundation for further spectral and statistical analysis.

## II. TIME EVOLUTION OF TRAJECTORY: SUPPLEMENTARY INFORMATION

In this section, we present supplementary information about the time evolution of the trajectory in Fig.2a in the main text. The trajectory is analyzed from the perspective of the frequency spectrum of kinetic energy in the main text. Here, following the spirit of Poincaré map, we further examine the crossing of the trajectory through a reference line for characterizing the aperiodic orbit.

The results are presented in Fig. 1. The crossing points of the trajectory (black curve) and the reference line (blue line) are indicated by red dots; the connecting line of the two furthest points in the trajectory is chosen as the reference line. With the increase of the time interval  $T$ , it is observed that crossing points proliferate and ultimately fill the entire reference line. Figure 1 demonstrates the filling of space in time by the aperiodic trajectory.

## III. FREQUENCY ANALYSIS: SUPPLEMENTARY CASES

In this section, we present supplementary information on the frequency spectrum analysis of kinetic energy, including the case of linear-spring system, sharpened pulses in the energy spectrum with the increase of the sampling interval, and the dynamical transition process from linear to nonlinear regime characterized by the proliferation and mixing of frequencies as the sampling interval increases.

### A. The case of linear-spring system

In this subsection, we present the main results of frequency analysis for the case of triplet system connected by linear springs. For comparison with the L-J particle system, the stiffness of the linear springs is set to be  $\beta_0$ , where  $\beta_0$  is the stiffness of the  $L - J$  potential at the equilibrium point.

Figure 2 shows the frequency spectra and trajectories of the disturbed triplet system

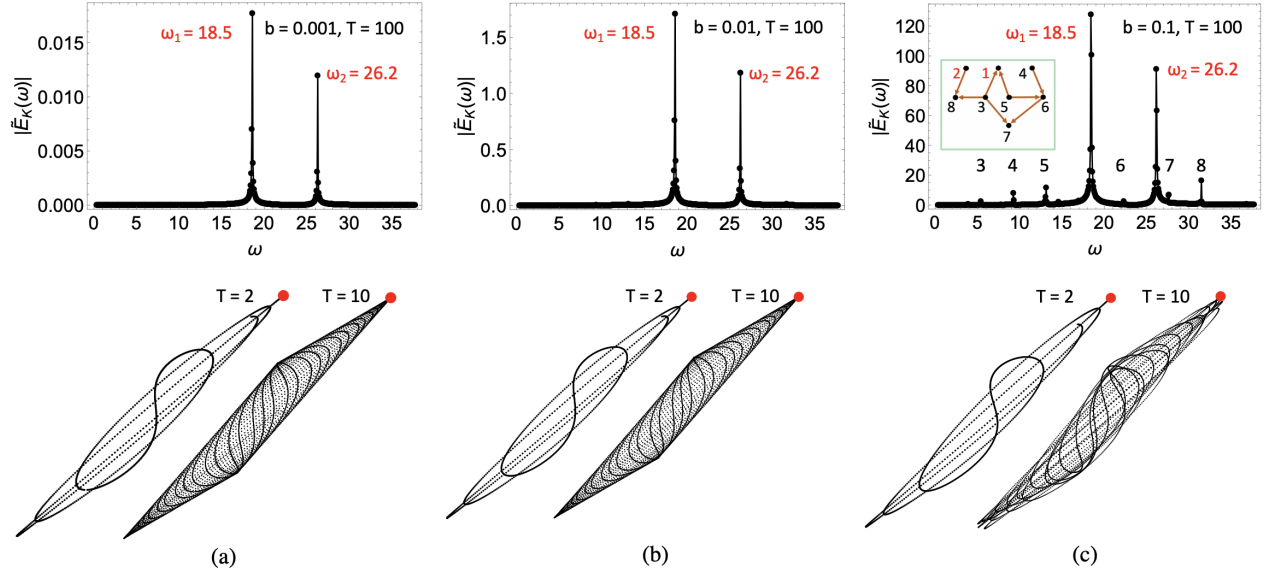

FIG. 2: Frequency analysis of the triplet system connected by linear springs under the same disturbance strength as in Fig.2 in the main text. The frequency spectra of the kinetic energy are obtained by discrete Fourier transformation. (a)-(c) The disturbance amplitude increases from 0.001 to 0.1, which correspond to Fig.2 in the main text. The relation of the emergent frequencies  $\omega_i$  in (c) is presented in the inset graph. The values for  $\omega_i$  in (c) are recorded here:  $\omega_3 = 5.4$ ,  $\omega_4 = 9.2$ ,  $\omega_5 = 13.1$ ,  $\omega_6 = 22.3$ ,  $\omega_7 = 27.7$ , and  $\omega_8 = 31.6$ . The trajectories are presented in the lower panels. The data are recorded in the sampling interval of  $t \in [0, T]$ .

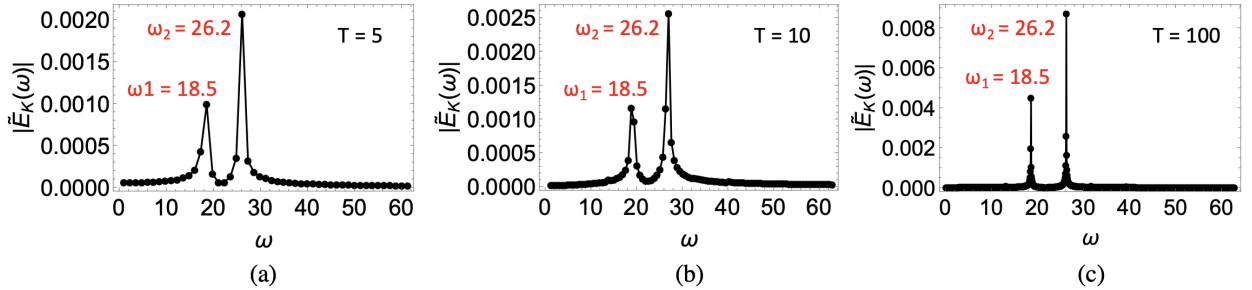

FIG. 3: Sharpening of the peaks in the spectra of the kinetic energy with the increase of the sampling interval  $T$ .  $t \in [0, T]$ . The positions of the peaks are invariant.  $b = 0.001$ .

connected by linear springs under the same disturbance strength as in Fig.2 in the main text. A pair of fundamental modes with the same frequencies as in the L-J system appear. The linear-spring system also exhibit frequency-mixing phenomenon with the increase of  $b$ . In comparison with the L-J system, the relative amplitudes of the emergent modes in

the linear-spring system are much smaller. The relation of the emergent frequencies  $\omega_i$  is presented in the inset graph in Fig. 2(c).

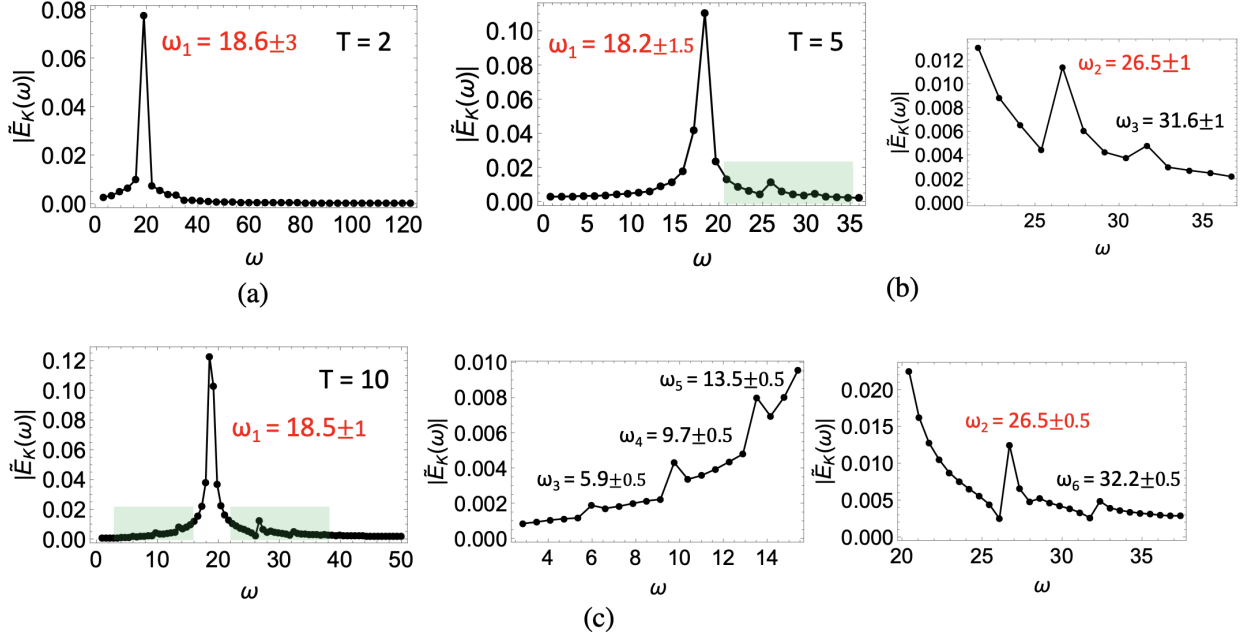

FIG. 4: Dynamical transition process from linear to nonlinear regime as characterized by the emergence of new frequencies with the increase of the sampling interval  $T$ . The intervals in the light green boxes are zoomed-in in the smaller figures. The  $\omega_1$  and  $\omega_2$  modes, which are indicated in red, are the two fundamental modes in the linear regime. The error on each indicated frequency is due to the width of the peak. The height of the peaks in (c) keeps growing with the increase of  $T$  up to  $T = 100$  [see Fig.2(b) in the main text].  $b = 0.01$ .

### B. Sharpened pulses in the energy spectrum with the increase of the sampling interval

In Fig. 3, we present the morphological change of the pulses in the spectrum of the kinetic energy with the increase of the sampling time interval  $T$ . The two pulses at the locations of the two fundamental frequencies at  $\omega_1 = 18.5$ , and  $\omega_2 = 26.2$  become sharpened when  $T$  increases from 5 to 100. Their positions are invariant.

### C. Dynamical transition from linear to nonlinear regime

Dynamical transition from linear to nonlinear regime occurs with the increase of the sampling interval  $T$ . Figure 4 shows the variation of the spectrum of the kinetic energy when  $T$  increases from 2 to 10 at  $b = 0.01$ . We see that the dynamical state of the system is dominated by the single mode of frequency  $\omega_1$  for  $T = 2$ , which is recognized as one of the two analytically derived fundamental modes in the linear regime. The other linear mode of frequency  $\omega_2$  arises when  $T$  reaches 5. Frequency-mixing process leads to the emergence of more frequencies in Fig. 4(c). With the increase of  $T$  up to 100, the amplitudes of all these frequencies grow to the level as in Fig.2(b) in the main text. This is an energy partition process among the modes.

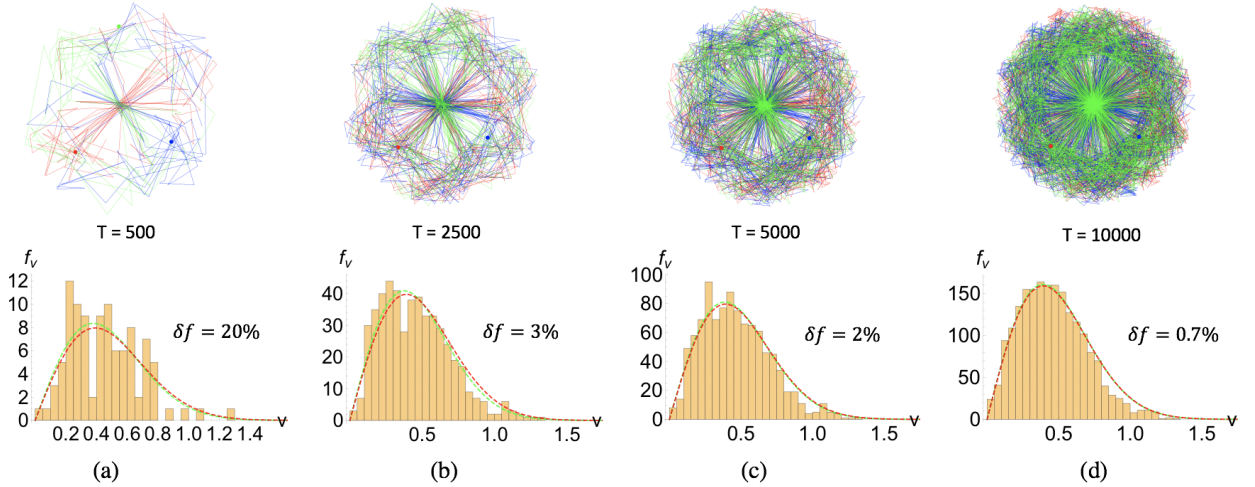

FIG. 5: Evolution of the speed distribution towards the Maxwell-Boltzmann distribution (indicated by the red dashed curve) with the increase of the sampling interval  $T$ .  $\delta f$  is a measure of the deviation between the numerically obtained speed distribution and the Maxwell-Boltzmann distribution. The optimal fitting curve for each histogram is shown in the green dashed curve. The associated trajectories of the particles are also presented in the upper array; the three particles are distinguished by different colors.

#### IV. STATISTICAL ANALYSIS: SUPPLEMENTARY CASES

In this section, we present supplementary information on the statistical analysis of particle trajectories, including the temporally-varying distribution of particle speed, and the spatial inhomogeneity revealed in the particle trajectories.

##### A. Temporally-varying distribution of instantaneous particle speed

In Fig. 5, we show the convergence of the speed distribution towards the two-dimensional Maxwell-Boltzmann distribution (indicated by the red dashed curve) with the increase of the sampling interval from  $T = 500$  [Fig. 5(a)] to  $T = 10000$  [Fig. 5(d)] corresponding to the case in Fig.3(c) in the main text. This asymptotic process is quantitatively characterized by

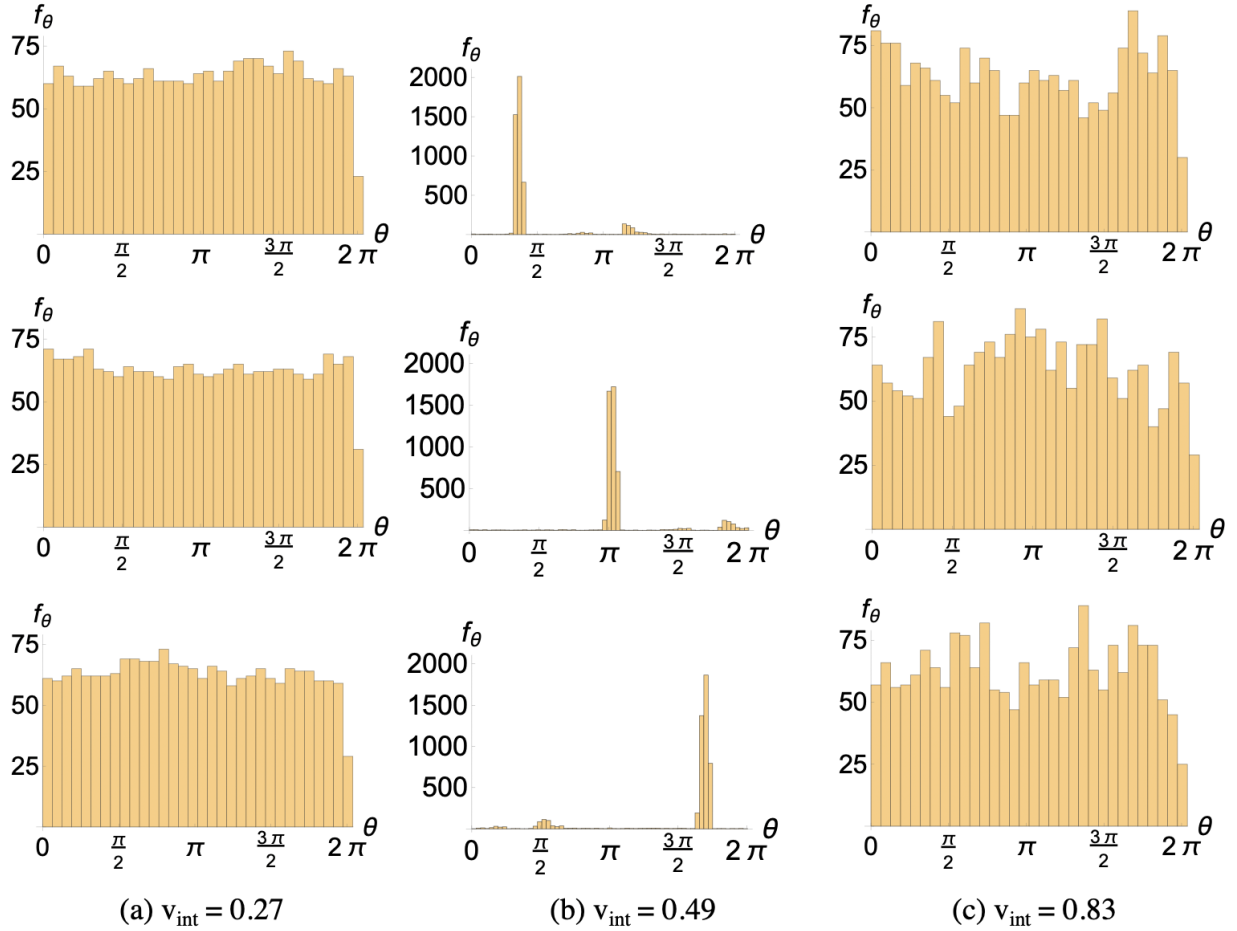

FIG. 6: Angular distribution of the recorded particle positions in the trajectories in Figs.3(a)-3(c) in the main text. Each array is for one of the three particles.

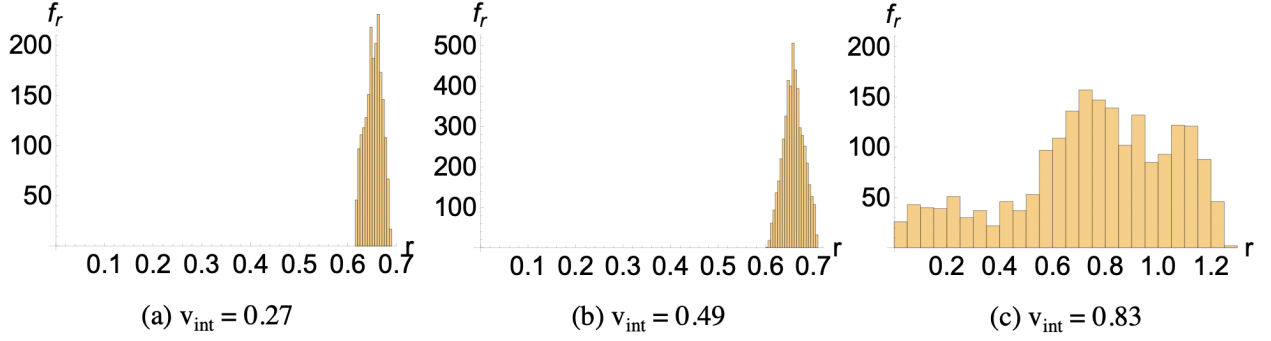

FIG. 7: Radial distribution of the recorded particle positions in the trajectories in Figs.3(a)-3(c) in the main text. The distribution profiles of the other two particles are almost the same as the presented one.

the reduction of  $\delta f$ , which is the deviation of the numerically obtained speed distribution from the Maxwell-Boltzmann distribution (see main text for the definition of  $\delta f$ ). The associated trajectories of motion are also presented in Fig. 5, where the three particles are distinguished by different colors.

### B. Trajectory analysis: distribution of particle positions

The spatial distributions of the particle positions in their trajectories for the cases in Figs.3(a)-(c) in the main text are presented in Fig. 6 and Fig. 7 in SI, respectively. Figure 6 shows the angular distributions of the three particles in their individual trajectories. For the case of  $v_{\text{ini}} = 0.49$  in Fig. 6(b), the particles tend to spend significantly longer time in specific small angle intervals; the three peaks correspond to a regular triangle.

The radial distributions for one of the three particles in their individual trajectories at varying  $v_{\text{ini}}$  are presented in Fig. 7; the distribution profiles of the other two particles are almost the same. The evolution of the region of motion from an annulus to a filled circle, as shown in Fig.3(a) in the main text, is quantitatively analyzed here. Furthermore, Figs. 7(a) and 7(b) show that the particles tend to spend more time along the central line of the annulus, which correspond to the balance distance in the three-body L-J system. The minimum structure in the L-J potential is also responsible for the inhomogeneity in the

radial distribution for the case of larger initial speed as shown in Fig. 7(c).

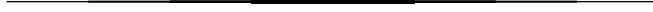

Supplement: Supplementary file 1 [file SI.pdf]
